# Supplementary material for: LoCoNet: Long-Short Context Network for Active Speaker Detection
Source: arXiv:2301.08237 source file (2024-03-29)
Supplement: Supplementary file 1 [file X_suppl.tex]

\clearpage
\setcounter{page}{1}
\maketitlesupplementary

\begin{figure*}
\centering
\includegraphics[width=0.9\textwidth]{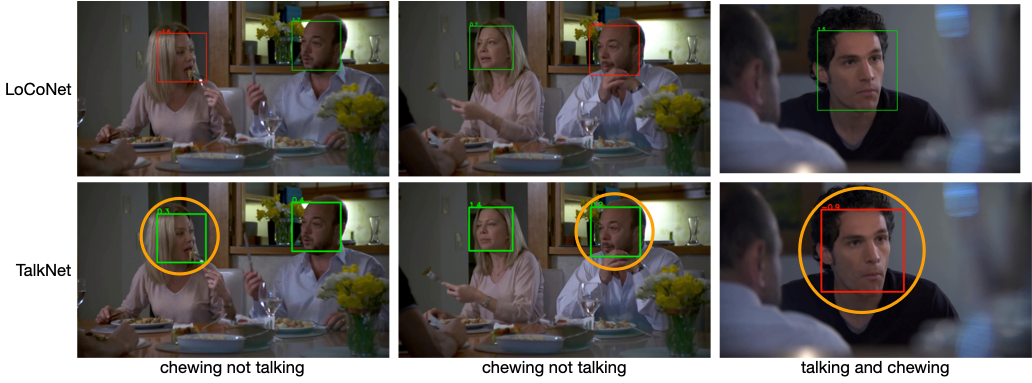}
\caption{\textbf{Results of \ModelName~and TalkNet on a video from AVA-ActiveSpeaker validation set.} The \textcolor{green}{green} boxes denote predicted active speaker. The \textcolor{red}{red} boxes denote predicted inactive speaker. The \textcolor{orange}{orange} boxes denote false predictions. This video shows a conversation on the dinner table, and the mouth movements of the speakers might be talking, chewing, or both.}
%\GB{I'm also quite confused about the figure. Based on the figure it seems that both short, and long-term context is modeling relationships with other speakers. I thought that one module was dedicated entirely for a target person. The font in the figure is also very small, which makes it difficult to see and reference parts mentioned in text.}
\label{fig:sup_ava}
%\vspace{-5pt}
\end{figure*}

\begin{figure*}
\centering
\includegraphics[width=0.9\textwidth]{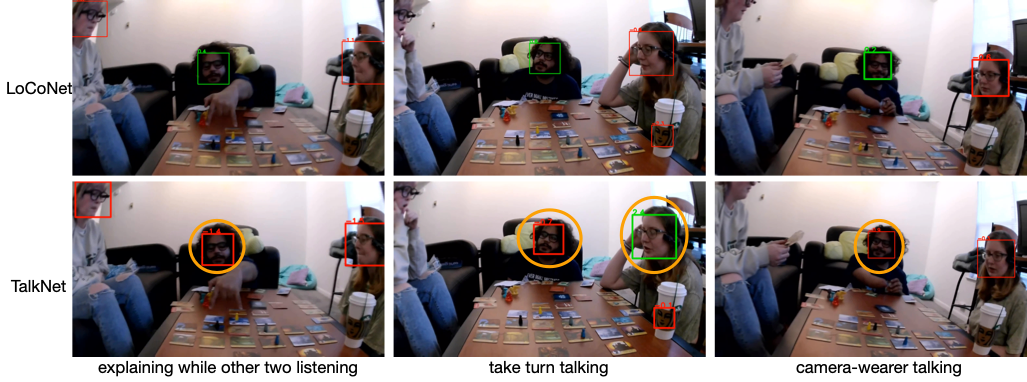}
\caption{\textbf{Results of \ModelName~and TalkNet~\cite{tao2021someone} on a video from Ego4D dataset.} This egocentric video shows a group of friends playing board games. The head motion of the camera-wearer and rapid shift in conversations make the inference more challenging.}
%\GB{I'm also quite confused about the figure. Based on the figure it seems that both short, and long-term context is modeling relationships with other speakers. I thought that one module was dedicated entirely for a target person. The font in the figure is also very small, which makes it difficult to see and reference parts mentioned in text.}
\label{fig:sup_ego}
%\vspace{-5pt}
\end{figure*}

\begin{figure*}
\centering
\includegraphics[width=0.9\textwidth]{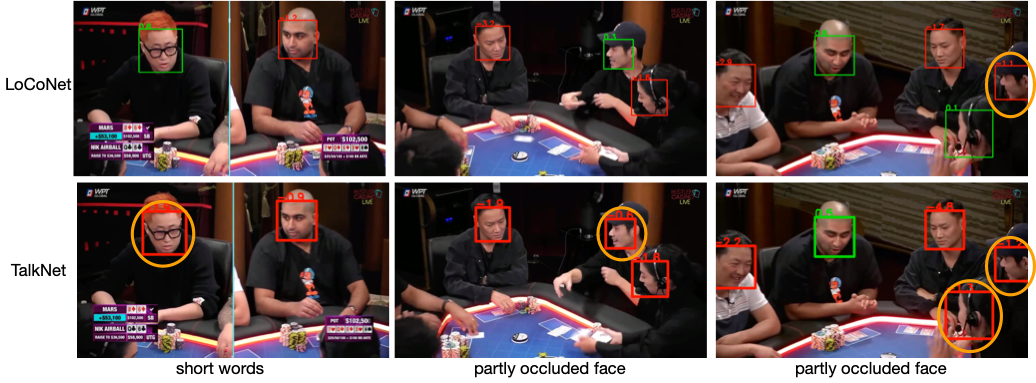}
\caption{\textbf{Results of \ModelName~and TalkNet~\cite{tao2021someone} on a video from the Internet.} This video shows a livestream of poker game with real-time narration. The results show that predicting speaking activities of a speaker with partly occluded face remains a difficult task.}
%\GB{I'm also quite confused about the figure. Based on the figure it seems that both short, and long-term context is modeling relationships with other speakers. I thought that one module was dedicated entirely for a target person. The font in the figure is also very small, which makes it difficult to see and reference parts mentioned in text.}
\label{fig:sup_poker}
%\vspace{-5pt}
\end{figure*}

\section{Comparison of results of \ModelName~and TalkNet}
\label{sec:results}
We show more comparisons and results of \ModelName~and TalkNet~\cite{tao2021someone} on videos from AVA-ActiveSpeaker~\cite{roth2020ava}(Fig.\ref{fig:sup_ava}), Ego4D~\cite{grauman2022ego4d}(Fig.\ref{fig:sup_ego}) and the Internet(Fig.\ref{fig:sup_poker}). The videos depict several complicated scenes including (1) talking and chewing, (2) egocentric view with head motion, and (3) poker game with narration. Results show that \ModelName~better differentiates active and inactive speakers in these complex scenes with multi-people conversations.

\section{Visualizations of the results of \ModelName}
\label{sec:visualization}

We generate the prediction results of \ModelName~on the videos from AVA-ActiveSpeaker, Ego4D and the Internet, and show the visualizations of the results by mapping them to the original videos. The visualizations are attached as mp4 files in the supplementary material. In the videos, the \textcolor{green}{green} boxes denote active speakers. The \textcolor{red}{red} boxes denote inactive speakers. The numbers above the boxes are logits where those larger than 0 are predicted as active speakers, and those smaller than 0 are predicted as inactive speakers.

% 
%Having the supplementary compiled together with the main paper means that:
% 
%\begin{itemize}
%\item The supplementary can back-reference sections of the main paper, for example, we can refer to \cref{sec:intro};
%\item The main paper can forward reference sub-sections within the supplementary explicitly (e.g. referring to a particular experiment); 
%\item When submitted to arXiv, the supplementary will already included at the end of the paper.
%\end{itemize}
% 
%To split the supplementary pages from the main paper, you can use \href{https://support.apple.com/en-ca/guide/preview/prvw11793/mac#:~:text=Delete%20a%20page%20from%20a,or%20choose%20Edit%20%3E%20Delete).}{Preview (on macOS)}, \href{https://www.adobe.com/acrobat/how-to/delete-pages-from-pdf.html#:~:text=Choose%20%E2%80%9CTools%E2%80%9D%20%3E%20%E2%80%9COrganize,or%20pages%20from%20the%20file.}{Adobe Acrobat} (on all OSs), as well as \href{https://superuser.com/questions/517986/is-it-possible-to-delete-some-pages-of-a-pdf-document}{command line tools}.
